# Supplementary material for: Another phase transition in the Axelrod model
Source: arXiv:1612.02537 source file (2016-12-08)
Supplement: Supplementary file 1 [file axelrodqrphase_sm.pdf]

# Supplemental Material

## Another phase transition in the Axelrod model

Alex Stivala      Paul Keeler

December 8, 2016

**Melbourne School of Psychological Sciences, The University of Melbourne, 3010, Australia**

Alex Stivala (stivalaa@unimelb.edu.au)

**Weierstrass Institute, Berlin 10117, Germany**

Paul Keeler (keeler@wias-berlin.de)

## 1 Introduction

In this Supplemental Material, we show the derivation of the master equation described by Castellano et al. (2000), given by

$$\frac{dP_m(t)}{dt} = \sum_{k=1}^{F-1} \frac{k}{F} P_k(t) \left[ \delta_{m,k+1} - \delta_{m,k} + (g-1) \sum_{n=0}^F (P_n(t) W_{n,m}^{(k)}(t) - P_m(t) W_{m,n}^{(k)}(t)) \right], \quad (1)$$

and its simplification

$$\begin{aligned} \frac{dP_m(t)}{dt} = & \left[ \frac{m-1}{F} P_{m-1}(t) - \frac{m}{F} P_m(t) \right] \\ & + (g-1) \left[ P_{m-1}(t) W_{m-1,m}^{(k)}(t) - P_m(t) W_{m,m-1}^{(k)}(t) \right. \\ & \left. + P_{m+1}(t) W_{m+1,m}^{(k)}(t) - P_m(t) W_{m,m+1}^{(k)}(t) \right] \sum_{k=1}^{F-1} \frac{k}{F} P_k(t), \end{aligned} \quad (2)$$

where the zeroth differential equation is

$$\frac{dP_0(t)}{dt} = - \sum_{m=1}^F \frac{dP_m(t)}{dt}. \quad (3)$$

## 2 Derivation of differential equations

If  $k = F$  or  $k = 0$ , then by the dynamics of the Axelrod model no change can occur, hence why the first summation in the master equation excludes these two scenarios. To further understand the set of non-linear differential equations, we first consider just the left hand-side, which we see simplifies to

$$\sum_{k=1}^{F-1} \frac{k}{F} P_k(t) [\delta_{m,k+1} - \delta_{m,k}] = \frac{m-1}{F} P_{m-1}(t) - \frac{m}{F} P_m(t).$$

The term  $P_k(t)$  is the probability of selecting a bond of type  $k$ , while the probability of selecting one of these  $k$  features is  $k/F$ , so the probability of two events both happening is the product  $kP_k(t)/F$ . In light of this, if  $k = m-1$ , then a new bond of type  $m$  is created, due to a new common feature across the bond arising. Conversely, if  $k = m$ , then a bond of type  $m$  is removed, due to a new common feature across the bond arising.

We now see in the master equation a balance between creation and removal of bonds. But when such a transition occurs, either creation or removal, then it is possible to create or destroy common features across the bonds for all the other sites, by our assumptions, in the von Neumann neighborhood of the transitioned (or culturally influenced) site in the randomly chosen bond. This can occur to  $g(R) - 1$  different sites, since the lattice is infinite, and we have again a balance between creation and removal of common features across bonds. For each bond of the  $g(R) - 1$  sites, change can occur regardless of how many common features they share, which is reflected by the second summation in the master equation.

For each transition that occurs for the initially chosen bond, a bond (connected to the other neighborhood sites) with  $n$  common features may be influenced by the transition of original bond with  $k$  common features so the newly influenced bond now has  $m$  common features, where we recall that the probability of such a transition is denoted by  $W_{n,m}^{(k)}(t)$ . But under such a transition, the number of common features can only increase by one, decrease by

one, or remain the same, so we see that the right-hand side of the master equation becomes

$$(g-1) \sum_{n=1}^F (P_n(t)W_{n,m}^{(k)} - P_m(t)W_{m,n}^{(k)}(t)) = (g-1) \left( P_{m-1}(t)W_{m-1,m}^{(k)}(t) - P_m(t)W_{m,m-1}^{(k)}(t) \right. \\ \left. + P_{m+1}(t)W_{m+1,m}^{(k)}(t) - P_m(t)W_{m,m+1}^{(k)}(t) \right),$$

where the  $W_{m,m}^{(k)}(t)$  terms canceled each other out, while all the other values of  $W_{n,m}^{(k)}(t)$  equal zero; also see Van Kampen (1992, Chapter VI). This results in

$$\frac{dP_m(t)}{dt} = \left[ \frac{m-1}{F} P_{m-1}(t) - \frac{m}{F} P_m(t) \right] \\ + (g-1) \sum_{k=1}^{F-1} \frac{k}{F} P_k(t) \left[ P_{m-1}(t)W_{m-1,m}^{(k)}(t) - P_m(t)W_{m,m-1}^{(k)}(t) \right. \\ \left. + P_{m+1}(t)W_{m+1,m}^{(k)}(t) - P_m(t)W_{m,m+1}^{(k)}(t) \right]. \quad (4)$$

We now need to derive the transition probabilities  $W_{n,m}^{(k)}(t)$ , which we will see are independent of  $k$  in the mean-field analysis.

### 3 Derivation of $W_{n,m}^{(k)}(t)$

We consider three sites, which we simply refer to as the first, second and third sites. The first and second sites are connected by the first bond with  $k$  common features, while the second and third sites are connected by the second bond with  $n$  common features. We will consider the different types of bonds in terms of their common features. By the dynamics of the model, we know features will not change if the number of common features on the first bond is  $k = 0$  or  $k = F$ , so these two cases are excluded. We assume the first bond has  $k$  common features, where  $0 < k < F$ , while the second bond has  $n$  common features. For concreteness, we can assume without loss of generality that the culture vector of the first site is a zero vector  $(0, 0, \dots, 0)$  with length  $F$ , while the second site's culture vector is  $(0, \dots, \sigma_{k+1}, \dots, \sigma_F)$ , where  $\sigma_i \neq 0$  for  $i > k$ , which ensures that the first and the second sites have only  $k$  common features. Similarly, the third site has another cultural vector  $(\sigma'_1, \sigma'_2, \dots, \sigma'_F)$ , which we can describe with an index set  $I_n \subset \{1, \dots, F\}$ , so there are  $n$  elements such that  $\sigma'_i = \sigma_i$  for  $i \in I_n$ . In other words, there are  $n$  entries of the third culture vector that coincide with the entries of the second culture vector, resulting in  $n$  common features across the second bond.

We now assume another common feature is created across the first bond, so we set  $\sigma_{k+1} = 0$ , which may create or remove a common feature across the second bond or have no effect at all. If  $n = F$ , then  $\sigma'_i = 0$  for  $i = 1, \dots, k$  and  $\sigma'_i = \sigma_i$  for  $i > k$ , so a common trait across the second bond, corresponding to  $\sigma_{k+1}$  and  $\sigma'_{k+1}$ , must be removed, implying

$$W_{F,F-1}^{(k)}(t) = 1.$$

For  $n = 0$ , two possibilities exist: a new common feature is created if  $\sigma'_{k+1} = 0$ , which we will assume occurs with probability  $\rho(t) = \mathbb{P}(\sigma'_{k+1} = 0)$ , or no new feature is created, which occurs with probability  $1 - \rho(t)$ .

If  $0 < n < F$ , the new feature change will remove a common feature across the second bond if it corresponds to one of the  $n$  common features across the third bond. The probability of this event can be reasoned by first noting that there are in total  $\binom{n}{F}$  different ways to have the  $n$  common features on the second bond. But only one of those common features will be the  $(k+1)$ th one, meaning the other  $n-1$  common features can be arranged in  $\binom{n-1}{F-1}$  different ways. The ratio of these two numbers and the previous transition probabilities give the general expression

$$W_{n,n-1}^{(k)}(t) = \frac{\binom{F-1}{n-1}}{\binom{F}{n}} = \frac{n}{F}, \quad 0 \leq n \leq F.$$

Given that the above event does not happen, the number of common features across the second bond remains or increases by one, so then the probability of  $n$  becoming  $n+1$  is the probability of  $\sigma'_{k+1} = 0$ , which we assume is also given by  $\rho(t) = \mathbb{P}(\sigma'_{k+1} = 0)$ , since  $\sigma_{k+1} = 0$ , and  $\sigma'_{k+1} \neq 0$ , then  $n$  remains  $n$ , which leads to the remaining transition probabilities

$$W_{n,n}^{(k)}(t) = \left[1 - W_{n,n-1}^{(k)}(t)\right] [1 - \rho(t)], \quad W_{n,n+1}^{(k)} = \left[1 - W_{n,n-1}^{(k)}(t)\right] \rho(t), \quad 0 \leq n \leq F.$$

**Choice of  $\rho(t)$**  For  $\rho(t)$ , the original choice was

$$\rho(t) = \frac{1}{F} \sum_{k=1}^F k P_k(t),$$

which is the average fraction of common features across a randomly chosen bond. However,  $\rho$  may be set to a constant value, giving qualitatively the same results (Castellano et al., 2000). We note that the choice of  $\rho$  means that there is no dependence on  $k$  in the expressions for the transition probabilities, which simplifies the summation in the master equation.

### 3.1 Small $g$ analysis

When the coordination number  $g = 1$ , the nonlinear component of the differential equations (2) disappears giving a tractable coupled set of linear differential equations

$$\frac{dP_m(t)}{dt} = \frac{m-1}{F}P_{m-1}(t) - \frac{m}{F}P_m(t), \quad 1 \leq m \leq F, \quad (5)$$

which can be solved using standard techniques such as Laplace transforms. For  $F \geq 3$ , the first three solutions are

$$P_1(t) = P_1(0)e^{-t/F} \quad (6)$$

$$P_2(t) = P_1(0)[e^{-t/F} - e^{-2t/F}] + P_2(0)e^{-2t/F} \quad (7)$$

$$P_3(t) = P_1(0)[e^{-t/F} + 2e^{-2t/F} - e^{-3t/F}] + 2P_2(0)[e^{-2t/F} - e^{-3t/F}] + P_3(0)e^{-3t/F}. \quad (8)$$

Now there are naturally no changes induced from other feature updates, and then, for all  $m \geq 1$  the probability  $P_m$  will rapidly converge to zero, or in other words,  $P_0$  will rapidly converge to one. To ensure non-zero convergence of  $P_m$ , the nonlinear term

$$(g-1) \sum_{k=1}^{F-1} \frac{k}{F} P_k(t) \left[ P_{m-1}(t)W_{m-1,m}^{(k)}(t) - P_m(t)W_{m,m-1}^{(k)}(t) + P_{m+1}(t)W_{m+1,m}^{(k)}(t) - P_m(t)W_{m,m+1}^{(k)}(t) \right], \quad (9)$$

must be sufficiently large and positive, which can be achieved by suitably varying the parameters  $g$ ,  $F$ , or  $q$ , the last model parameter appearing only in the initial values  $P_m(0)$  of the differential equations.

## 4 Numerical solution

The numerical solution of the master equation was carried out using MATLAB®. The MATLAB® code is available from [https://sites.google.com/site/alexdstivala/home/axelrod\\_qrphase/](https://sites.google.com/site/alexdstivala/home/axelrod_qrphase/).

## References

- Claudio Castellano, Matteo Marsili, and Alessandro Vespignani. Nonequilibrium phase transition in a model for social influence. *Phys. Rev. Lett*, 85(16):3536–3539, 2000.
- Nicolaas Godfried Van Kampen. *Stochastic processes in physics and chemistry*, volume 1. Elsevier, 1992.
